# Supplementary material for: Convolution-enhanced Evolving Attention Networks
Source: arXiv:2212.08330 source file (2023-04-28)
Supplement: Supplementary file 2 [file appendix.tex]

\appendix

%\section*{Quality of Image Attention}
%We select the 16th, 17th and 18th attention layers in the AA-ResNet-34 and EA-AA-ResNet34 networks for analysis. The attention maps from these layers have a shape of $14 \times 14 \times 8$, where 14 is the image length after pooling and 8 is the number of heads. Then, we send the attention maps directly as inputs to another CNN model for classification, and the original labels are used for training and evaluation. The goal is to quantify the effectiveness of attention maps learned by different models. If an attention map retains major structures of the original object, the classification accuracy should be higher. We adopt a 12-layer DenseNet~\cite{huang2017densely} for attention map classification, while the shape is pooled to $7 \times 7$ and $4 \times 4$ after the 4th and 7th layers respectively. The hidden dimension is set as 256 initially and doubled after each pooling operation. The models are trained by 30 epochs with cosine learning rate decay started by 0.05 and ended by 0.0001.

%\section*{Interpretability}

\section*{Visualization of Attention Maps}
We compare the attention maps of AA-ResNet-34 and EA-AA-ResNet-34 for some image classification cases.
Note that the number of heads in all models is set as 8 for image classification tasks. 
In Figure 1 and 5, we choose the best head in each layer to visualize the corresponding attention map, while the attention maps for all heads are visualized in the Figure 10-13.

Compared to AA-ResNet, our proposed convolution-based evolving attention mechanism captures better global information and at the same time emphasizes on the important local information. Specifically, the residual connections and convolutional inductive bias assist the self-attention mechanism to depict a more clear outline. As shown by the visualized examples, AA-ResNet fails to compute the explainable attention maps for some layers. In contrast, with the help of residual convolutions, EA-AA-ResNet successfully identifies the objects in images in an evolving process.

\begin{figure*}[t]
     \begin{center}
        \includegraphics[width=1.0\linewidth]{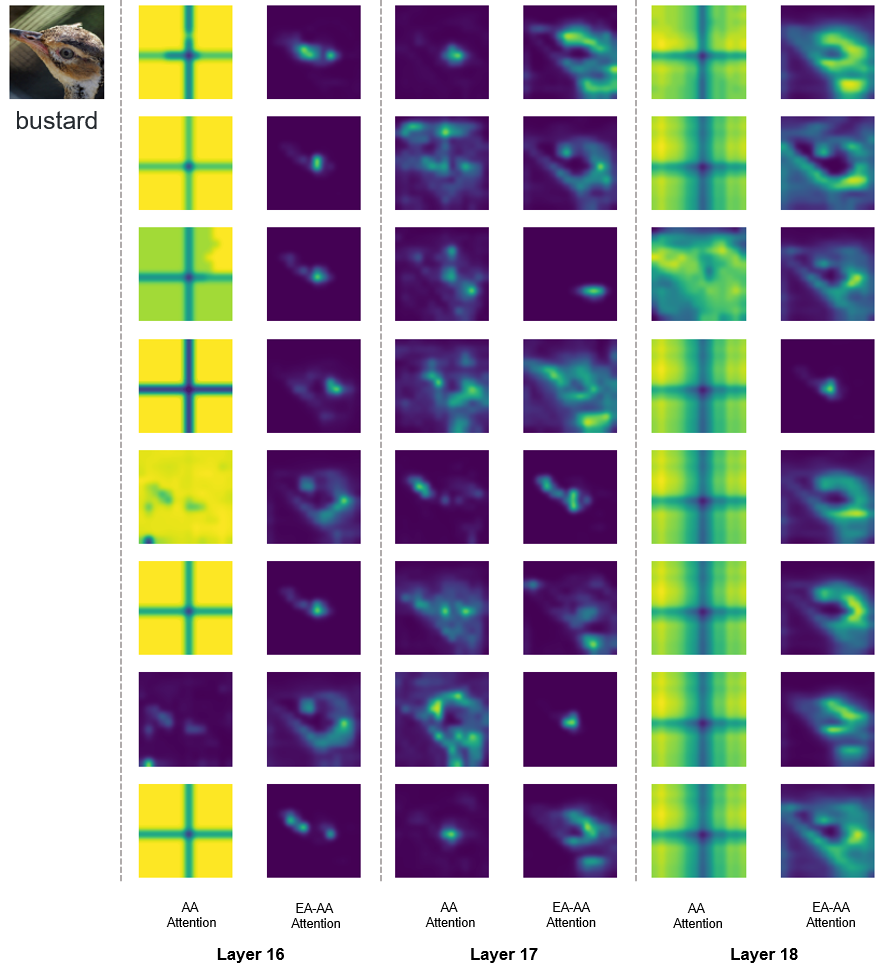}
     \end{center}
      \caption{Attention map visualization of all 8 heads for an image classification example}
      \label{fig:bird_attention0}
\end{figure*}

\begin{figure*}[t]
     \begin{center}
        \includegraphics[width=1.0\linewidth]{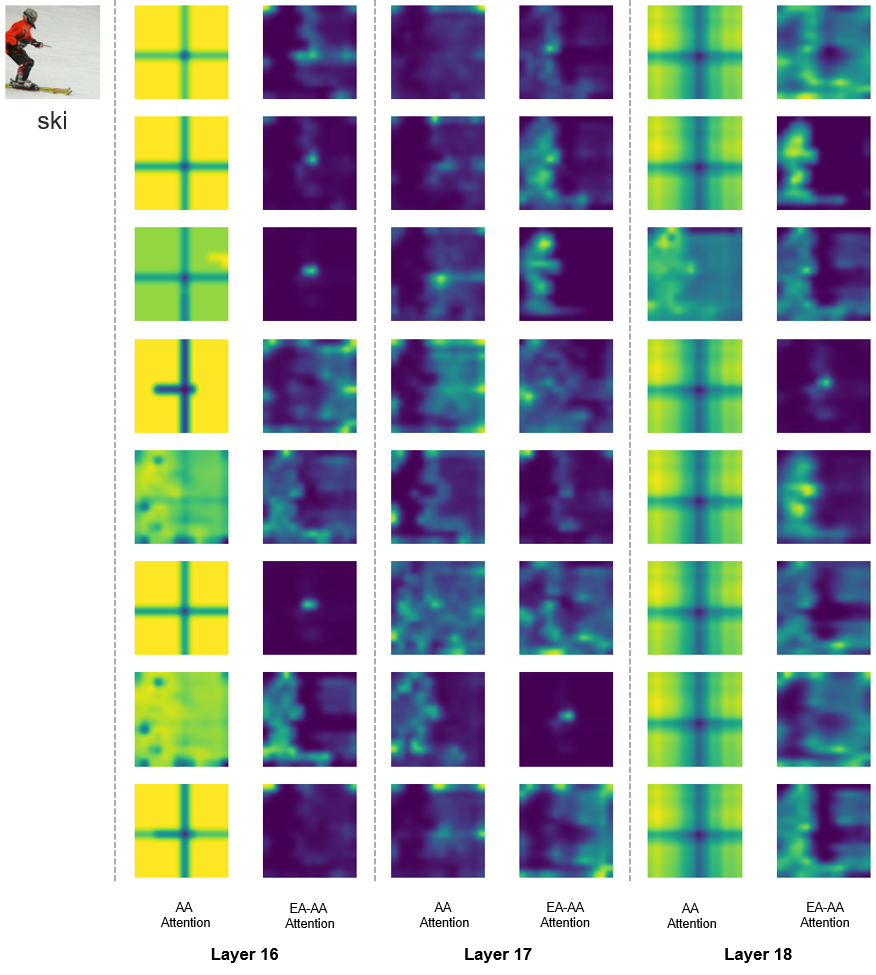}
     \end{center}
      \caption{Attention map visualization of all 8 heads for an image classification example}
      \label{fig:bird_attention1}
\end{figure*}

\begin{figure*}[t]
     \begin{center}
        \includegraphics[width=1.0\linewidth]{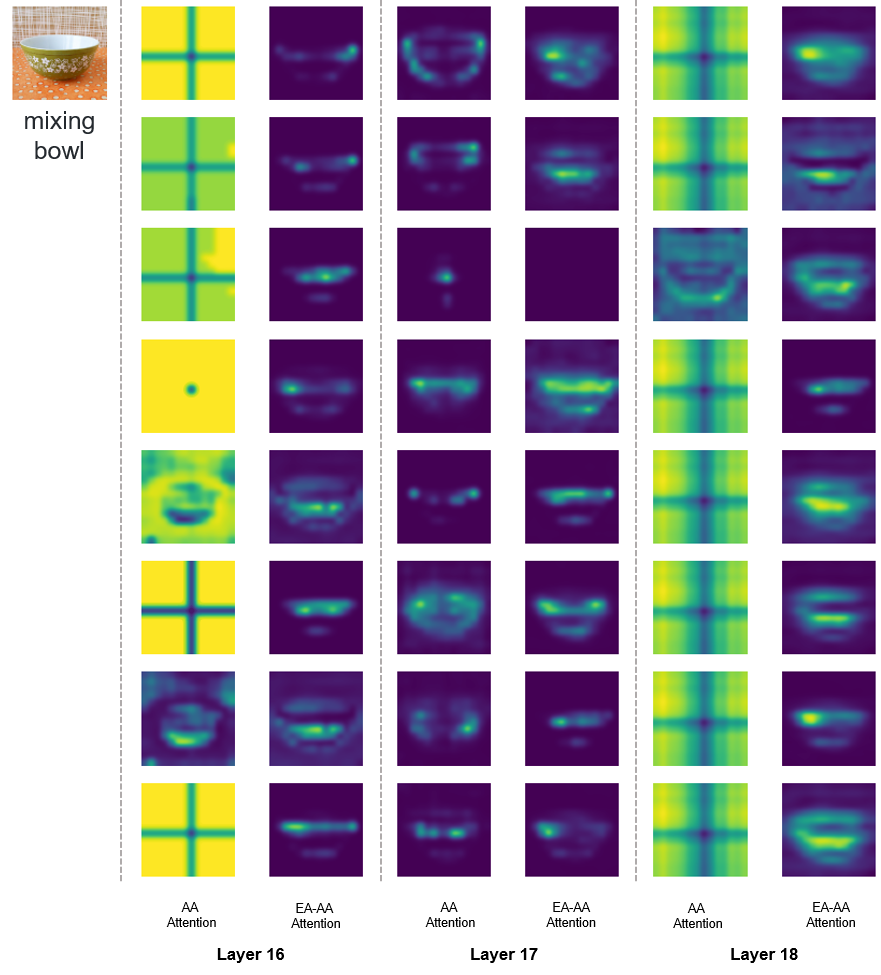}
     \end{center}
      \caption{Attention map visualization of all 8 heads for an image classification example}
      \label{fig:bird_attention2}
\end{figure*}

\begin{figure*}[t]
     \begin{center}
        \includegraphics[width=1.0\linewidth]{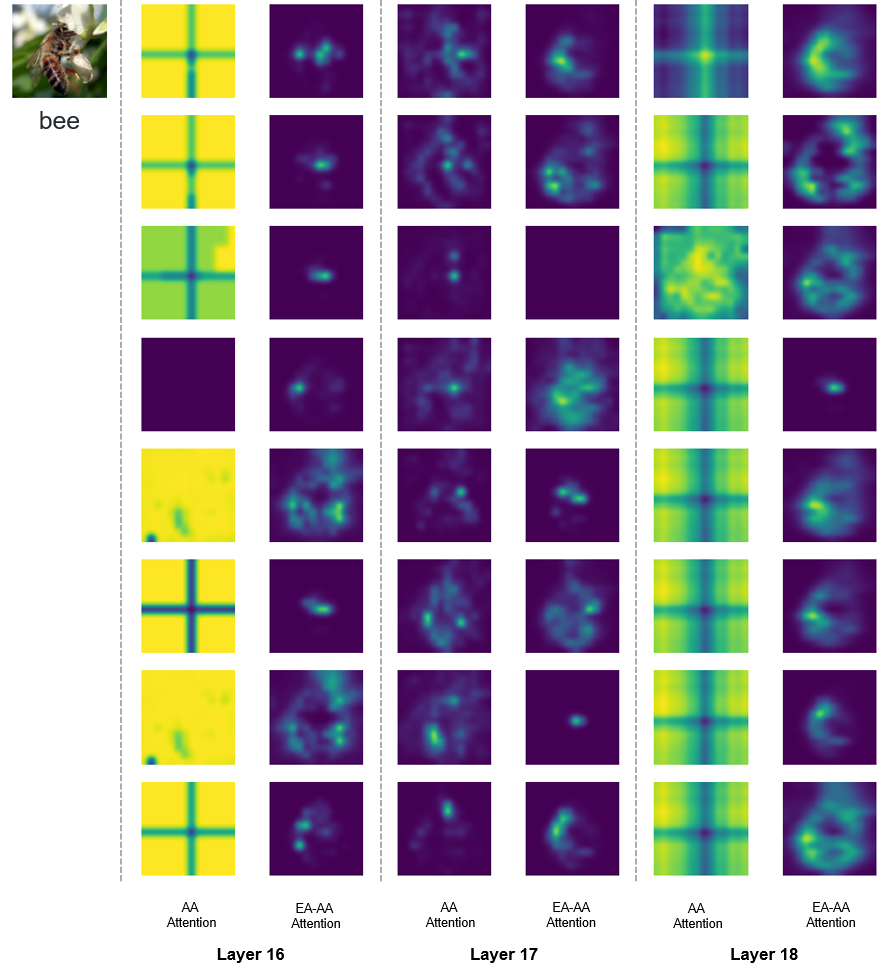}
     \end{center}
      \caption{Attention map visualization of all 8 heads for an image classification example}
      \label{fig:bird_attention3}
\end{figure*}

\section*{Hyper-parameter settings}

\subsection*{Hyper-parameters of EA-DC-Transformer}
By default, we use 3-fold cross validation for hyper-parameter selection. 
% We randomly select 30\% of the training set as the valid set to compare the performance when applying different settings. 
We randomly select 30\% of the training set as the valid set, and compare the performance in different settings by taking the average of valid set results in 3-fold experiments as the metric for hyper-parameter selection.
As for how to search for hyper-parameters concretely, we give an example of searching hidden dimension in the following\footnote{\url{https://github.com/lizzylizzylizzy/EvolvingAttention/blob/master/EA_DC_Transformer/src/main.py\#L429}}. For each hyper-parameter setting, we will record the model performance results line by line in an excel book. The path of the specific excel file is set through the argument
 \textit{records\_file}. Then we can select the most appropriate hyper-parameter configuration according to the average results of the valid set recorded in the excel file, and report its corresponding evaluation metrics on the test set. 
In our experiments, hyper-parameters for EA-DC-Transformer are tuned in the following search space: hidden dimension \{64, 128\}, $\alpha=$\{0.1, 0.3, 0.5, 0.7, 0.9\} and $\beta=$\{0.1, 0.3, 0.5, 0.7, 0.9\}. 
The dimension ratio to combine convolution and transformer branches is chosen from $p=$\{0.125, 0.25, 0.375, 0.5, 0.625, 0.75, 0.875\}. 
The number of blocks $n$ is chosen from \{2, 3, 4, 5\}. 
We adopt Rectified Adam optimizer~\cite{liu2019variance} with $\beta_1 = 0.9$ and $\beta_2 = 0.99$. The dropout ratio is 0.1, and the learning rate is set to 1e-3 empirically. 

 \subsection*{Hyper-parameters of EA-ViT models}

One can refer to Table~\ref{tab:ea_vit_hyp} for specific hyper-parameter settings of all EA-ViT models.

\begin{table}
\centering
\caption{Hyper-parameters of EA-ViT models}
\scalebox{0.8}{
    
    \begin{tabular}{ccccc}
    \toprule
     \textbf{Hyper-parameter} & \textbf{EA-ViT/B-32} & \textbf{EA-ViT/B-16} & \textbf{EA-ViT/L-32} & \textbf{EA-ViT/L-16} \\ 
     \midrule
     Steps & 20000 & 20000 & 20000 & 20000 \\
     Batch size & 512 & 512 & 512 & 512 \\
     Base LR & 0.03 & 0.03 & 0.03 & 0.03 \\
     Dropout & 0.1 & 0.1 & 0.1 & 0.1 \\
     $\alpha$ & 0.1 & 0.1 & 0.1 & 0.1  \\
     $\beta$ & 0.3 & 0.3 & 0.3 & 0.3 \\
     \bottomrule
    \end{tabular}
}
    \label{tab:ea_vit_hyp}
\end{table}

\subsection*{Hyper-parameters of Other EA-enhanced models}

For the hyper-parameters of other EA-enhanced models, including EA-AA-ResNet, EA-Transformer, EA-BERT, EA-T5, and EA-RoBERTa, one can refer to the Appendix in the ICML paper\footnote{\url{https://arxiv.org/abs/2102.12895}}.
